# Supplementary material for: The multi-channel Dyson equation: coupling many-body Green's functions
Source: arXiv:2310.01204 source file (2023-10-02)
Supplement: Supplementary file 1 [file supmat.pdf]

# Supplemental Material to "The multi-channel Dyson equation: coupling many-body Green's functions"

Gabriele Riva,[1] Pina Romaniello,[2] and J. Arjan Berger[1]

[1]*Laboratoire de Chimie et Physique Quantiques, Université de Toulouse, UPS, CNRS, and European Theoretical Spectroscopy Facility (ETSF), 118 route de Narbonne, F-31062 Toulouse, France*

[2]*Laboratoire de Physique Théorique, CNRS, Université de Toulouse, UPS, and European Theoretical Spectroscopy Facility (ETSF), 118 route de Narbonne, F-31062 Toulouse, France*

## REMINDER OF THE FEYNMAN RULES

In the main text as well as in the next section we will use Feynman diagrams. Therefore, in the following, we briefly recall the Feynman rules.

1. Each vertex represents a spin-position coordinate $x_i$
2. Each solid line with an arrow represents a non-interacting 1-GF
3. Each wiggly line represents a bare Coulomb interaction
4. Each dotted line represent a Dirac delta function
5. Internal lines are integrated over position and summed over spin
6. For each 1-GF diagram there is a prefactor $(-1)^F i^n$ where $F$ is the number of closed fermion loops, and $n$ is the order in the Coulomb interaction.

## DIAGRAMMATIC ANALYSIS OF THE MULTI-CHANNEL DYSON EQUATION

To analyze in more detail the diagrammatic structure of the multi-channel Dyson, we start by writing the multi-channel self-energy in real space. For completeness, we first report the equations in orbital space which we have already given in the main manuscript

$$\begin{aligned}\Sigma^{\text{3p}}_{ijl;mok} &= [(1-f_i)(1-f_j)f_l - f_i f_j(1-f_l)][\delta_{lk}\bar{v}_{ijom} \\ &\quad + \delta_{mj}\bar{v}_{iklo} + \delta_{io}\bar{v}_{jklm} - \delta_{oj}\bar{v}_{iklm} - \delta_{im}\bar{v}_{jklo}] \quad (1)\\ \Sigma^{\text{c}}_{i;mok} &= \bar{v}_{ikom} \quad (2)\\ \tilde{\Sigma}^{\text{c}}_{ijl;m} &= \bar{v}_{ijlm} \quad (3)\end{aligned}$$

for which we have used the following change of basis

$$\begin{aligned}\Sigma^{\text{3p}}_{ijl;mok} &= \int dx_1 dx_2 dx_3 dx_{1'} dx_{2'} dx_{3'} \Sigma^{\text{3p}}(x_1, x_2, x_{3'}, x_{1'}, x_{2'}, x_3) \quad (4)\\ &\quad \times \phi^*_i(x_1)\phi^*_j(x_2)\phi_l(x_{3'})\phi_m(x_{1'})\phi_o(x_{2'})\phi^*_k(x_3), \\ \Sigma^{\text{c}}_{i;mok} &= \int dx_1 dx_3 dx_{1'} dx_{2'} \Sigma^{\text{c}}(x_1, x_{1'}, x_{2'}, x_3) \quad (5)\\ &\quad \times \phi^*_i(x_1)\phi_m(x_{1'})\phi_o(x_{2'})\phi^*_k(x_3), \\ \tilde{\Sigma}^{\text{c}}_{ijl;m} &= \int dx_1 dx_2 dx_{1'} dx_{3'} \tilde{\Sigma}^{\text{c}}(x_1, x_2, x_{3'}, x_{1'}) \quad (6)\\ &\quad \times \phi^*_i(x_1)\phi^*_j(x_2)\phi_l(x_{3'})\phi_m(x_{1'}).\end{aligned}$$

The multi-channel self-energy is

$$\begin{aligned}\Sigma^{2e1h}(x_1, x_2, x_{3'}, x_{1'}, x_{2'}, x_3) &= -\Sigma^{2h1e}(x_1, x_2, x_{3'}, x_{1'}, x_{2'}, x_3) \\ &= \delta(x_3, x_{3'})[\delta(x_1, x_{1'})\delta(x_2, x_{2'}) - \delta(x_1, x_{2'})\delta(x_2, x_{1'})]v(\mathbf{r}_1, \mathbf{r}_2) \\ &+ \delta(x_{1'}, x_2)[\delta(x_1, x_{2'})\delta(x_3, x_{3'}) - \delta(x_1, x_{3'})\delta(x_3, x_{2'})]v(\mathbf{r}_1, \mathbf{r}_3) \quad (7)\\ &+ \delta(x_1, x_{2'})[\delta(x_2, x_{1'})\delta(x_3, x_{3'}) - \delta(x_2, x_{3'})\delta(x_3, x_{1'})]v(\mathbf{r}_2, \mathbf{r}_3) \\ &- \delta(x_2, x_{2'})[\delta(x_1, x_{1'})\delta(x_3, x_{3'}) - \delta(x_1, x_{3'})\delta(x_3, x_{1'})]v(\mathbf{r}_1, \mathbf{r}_3) \\ &- \delta(x_1, x_{1'})[\delta(x_2, x_{2'})\delta(x_3, x_{3'}) - \delta(x_2, x_{3'})\delta(x_3, x_{2'})]v(\mathbf{r}_2, \mathbf{r}_3) \\ \Sigma^{\text{c}}(x_1, x_{1'}, x_{2'}, x_3) &= [\delta(x_1, x_{1'})\delta(x_{2'}, x_3) - \delta(x_1, x_{2'})\delta(x_{1'}, x_3)]v(\mathbf{r}_1, \mathbf{r}_3) \quad (8)\\ \tilde{\Sigma}^{\text{c}}(x_1, x_2, x_{3'}, x_{1'}) &= [\delta(x_1, x_{1'})\delta(x_2, x_{3'}) - \delta(x_1, x_{3'})\delta(x_2, x_{1'})]v(\mathbf{r}_1, \mathbf{r}_2). \quad (9)\end{aligned}$$

From these expressions in real space it becomes easier to understand the diagrammatic structure. The body is

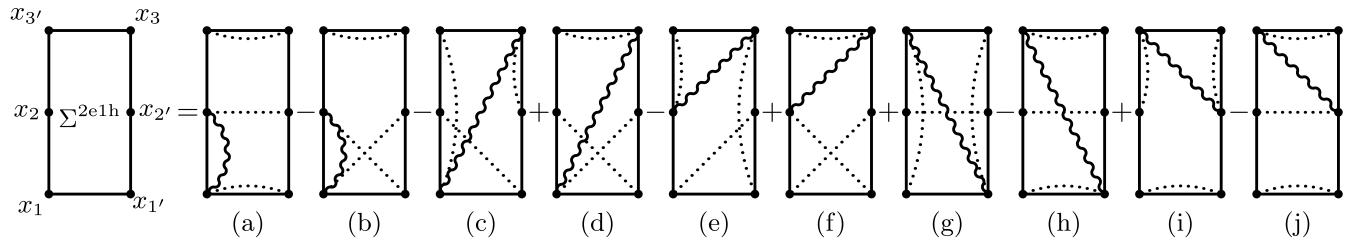


and the coupling terms are

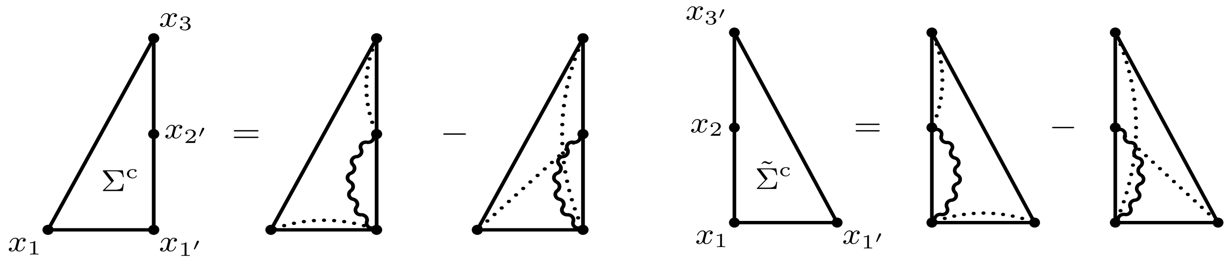


Now we show how to calculate a second-order self-energy diagram from the multi-channel Dyson equation. We choose the following example

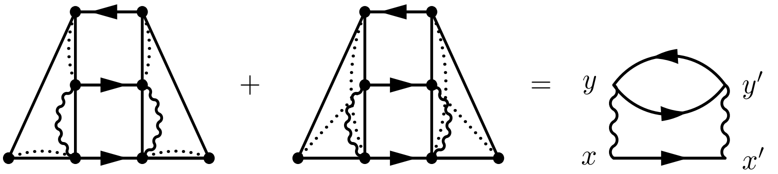 (10)


From the standard diagrammatic theory, the diagram on the right-hand side is defined by the equation

$$\Sigma(xt, x't') = G^0(xt, x't') \int dydy' v(\mathbf{x}, \mathbf{y}) v(\mathbf{x'y'}) G^0(yt, y't') G^0(y't', yt). \tag{11}$$

Fourier transforming to the frequency domain, with $G_{01}(x, x'; \omega) = \sum_n \frac{\phi_n(x)\phi_n^*(x')}{\omega - \epsilon_n + i\eta \mathrm{sign}(\epsilon_n - \mu)}$, this self-energy becomes

$$\begin{aligned}\Sigma(x, x', \omega) = &\int dydy' v(\mathbf{x}, \mathbf{y}) v(\mathbf{x'y'}) [\sum_{\substack{vcc' \\ c' \neq c}} \frac{\phi_c(x)\phi_c^*(x')\phi_{c'}(y)\phi_{c'}^*(y)\phi_v(y')\phi_v^*(y)}{\omega - \epsilon_c - (\epsilon_{c'} - \epsilon_v) + i\eta} \\ &+ \sum_{\substack{cvv' \\ v' \neq v}} \frac{\phi_v(x)\phi_v^*(x')\phi_{v'}(y)\phi_{v'}^*(y)\phi_c(y')\phi_c^*(y)}{\omega - \epsilon_v + (\epsilon_c - \epsilon_{v'}) - i\eta}],\end{aligned} \tag{12}$$

where $v$ and $c$ stand for valence and conduction states, respectively. Finally, using the basis that diagonalizes $G_{01}$, and the relation $v_{ijlm} = \int dx_1 dx_2 \phi_i^*(x_1)\phi_j^*(x_2) v(\mathbf{r}_1, \mathbf{r}_2)\phi_l(x_2)\phi_m(x_1)$ we obtain

$$\begin{aligned}\Sigma_{im}(\omega) &= \int dxdx' \phi_i(x)^* \phi_m(x') \Sigma(x, x', \omega) \\ &= \sum_{\substack{vcc' \\ c' \neq c}} \frac{v_{ivcc'} v_{c'cvm}}{\omega - \epsilon_{c'} - (\epsilon_c - \epsilon_v) + i\eta} + \sum_{\substack{cvv' \\ v' \neq v}} \frac{v_{icvv'} v_{vv'mc}}{\omega - \epsilon_{v'} - (\epsilon_v - \epsilon_c) - i\eta}.\end{aligned} \tag{13}$$

Let us now analyze the diagrams that we obtained with the multi-channel Dyson equation. The total second-order proper self-energy is calculated as

$$
\begin{aligned}
\Sigma_{im}^{second} &= \sum_{\substack{m'o'k' \\ i''j''l'' \\ m'>o',i''>j''}} \Sigma^{coupling}_{i,m'o'k'} G^{3p}_{03(m'o'k';i''j''l'')}(\omega)\tilde{\Sigma}^{coupling}_{i''j''l'',m} \\
&= \sum_{\substack{m'o'k' \\ i''j''l'' \\ m'>o',i''>j''}} \bar{v}_{ik'o'm'} \frac{\delta_{m'i''}\delta_{o'j''}\delta_{k'l''}(f_{m'}-f_{k'})(f_{o'}-f_{k'})}{\omega-\epsilon_{m'}-(\epsilon_{o'}-\epsilon_{k'})+i\eta\,\mathrm{sign}(1/2-f_{m'})}\bar{v}_{i''j''l''m} \\
&= \sum_{\substack{vcc', \\ c>c'}} \frac{\bar{v}_{ivcc'}\bar{v}_{c'cvm}}{\omega-\epsilon_{c'}-(\epsilon_c-\epsilon_v)+i\eta} + \sum_{\substack{cvv', \\ v>v'}} \frac{\bar{v}_{icvv'}\bar{v}_{v'vcm}}{\omega-\epsilon_{v'}-(\epsilon_v-\epsilon_c)-i\eta}.
\end{aligned}
\tag{14}
$$

For the last equality, we divide the space in valence and conduction state using the conditions $(f_{m'}-f_{k'})(f_{o'}-f_{k'})$.

Here all the combinations of the coupling terms are taken into account. To get the expressions which correspond to the two diagrams on the left-hand side of Eq.(10) we have to choose both potentials direct or both inverse ($\bar{v} = v^{direct} - v^{inverse}$). Looking at the first term in the last row of Eq.(14), this means that we have only the following term

$$
\begin{aligned}
\sum_{\substack{vcc' \\ c>c'}} \frac{v_{ivcc'}v_{c'cvm}+v_{ivc'c}v_{c'cmv}}{\omega-\epsilon_{c'}-(\epsilon_c-\epsilon_v)+i\eta} &= \sum_{\substack{vcc' \\ c>c'}} \frac{v_{ivcc'}v_{c'cvm}}{\omega-\epsilon_{c'}-(\epsilon_c-\epsilon_v)+i\eta} \\
+\sum_{\substack{vcc' \\ c<c'}} \frac{v_{ivcc'}v_{cc'mv}}{\omega-\epsilon_{c}-(\epsilon_{c'}-\epsilon_v)+i\eta} &= \sum_{\substack{vcc' \\ c'\neq c}} \frac{v_{ivcc'}v_{c'cvm}}{\omega-\epsilon_{c'}-(\epsilon_c-\epsilon_v)+i\eta},
\end{aligned}
\tag{15}
$$

where in the first equality, the second term is obtained using $c \leftrightarrow c'$ for the second term in the numerator, and to obtain the last term the relation $v_{cc'vm} = v_{c'cmv}$ is used. For the second term in the last row of Eq.(14) the same argument holds.

Therefore, we finally obtain

$$
\Sigma_{im}(\omega) = \sum_{\substack{vcc' \\ c'\neq c}} \frac{v_{ivcc'}v_{c'cvm}}{\omega-\epsilon_{c'}-(\epsilon_c-\epsilon_v)+i\eta} + \sum_{\substack{cvv' \\ v'\neq v}} \frac{v_{icvv'}v_{vv'mc}}{\omega-\epsilon_{v'}-(\epsilon_v-\epsilon_c)-i\eta}
\tag{16}
$$

that is the same expression as (13), namely the exact result for one of the two second-order diagrams.

Along the same lines, it is possible to verify that the multi-channel Dyson equation gives also the exact third order proper skeleton diagrams. To show in a more clear way that, at third order, we need four different self-energy combinations to obtain a single $\Sigma_1$ diagram we report the following example

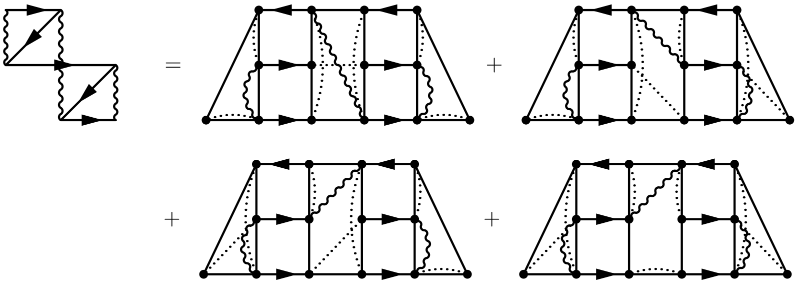

When two $G_{01}$ line merge without interacting, the following identity has to be used

$$
G^0_{im}(t-t') = i\sum_l G^{0(e)}_{il}(t-t'')G^{0(e)}_{lm}(t''-t') - i\sum_l G^{0(h)}_{il}(t-t'')G^{0(h)}_{lm}(t''-t'),
\tag{17}
$$

where the definition $G^0_{im}(t) = G^{0(e)}_{im}(t) + G^{0(h)}_{im}(t)$ is used.

## HUBBARD DIMER CALCULATION

Here, we report the solution of the multi-channel Dyson equation for the Hubbard dimer. We do the analysis in the bonding (b) and anti-bonding (a) basis, in which the non-interacting term is diagonal. In this basis the Coulomb potential is given by

$$v^{b/a}_{ijlm} = \frac{U}{2}\delta_{\sigma_i\sigma_m}\delta_{\sigma_j\sigma_l}(\delta_{\tilde{i}\tilde{m}}\delta_{\tilde{j}\tilde{l}} + \delta_{\tilde{i}\tilde{j}}\delta_{\tilde{m}\tilde{l}} + \delta_{\tilde{i}\tilde{l}}\delta_{\tilde{j}\tilde{m}} - 2\delta_{\tilde{i}\tilde{m}}\delta_{\tilde{j}\tilde{l}}\delta_{\tilde{i}\tilde{j}}). \tag{18}$$

where $U$ is the on-site interaction, $i = \{\sigma_i\tilde{i}\}$ specifies the orbital $\tilde{i}$ with spin $\sigma_i$, and $\tilde{i}$ is equal to bonding or anti-bonding.

The exact expressions of the 1-GF and the 3-GF can be found in [1], and [2], respectively. Therefore, in the following, we will focus on the 1-GF and 3-GF obtained with our approximate multi-channel self-energy.

### 1/4 filling

The non-interacting (HF) 3-GF is given by

$$\begin{aligned} G_{03}(\omega) = \text{Diag}\Big[&\frac{1}{\omega-(\epsilon_0-t)-i\eta}, \frac{1}{\omega-(\epsilon_0-t+\frac{U}{2})+i\eta}, \frac{1}{\omega-(\epsilon_0+t+\frac{U}{2})+i\eta}, \frac{1}{\omega-(\epsilon_0+t)+i\eta}, \\ &\frac{1}{\omega-(\epsilon_0+3t+\frac{U}{2})+i\eta}, \frac{1}{\omega-(\epsilon_0+t+U)+i\eta}, \frac{1}{\omega-(\epsilon_0+t+\frac{U}{2})+i\eta}\Big], \end{aligned} \tag{19}$$

where the first three elements are from the 1-GF with $i = b\uparrow; b\downarrow; a\downarrow; a\uparrow$, respectively, and the last three are from $G^{3\text{p}}_{03}$ with $ijl = (a\downarrow a\uparrow b\uparrow); (a\downarrow b\downarrow b\uparrow); (a\uparrow b\downarrow b\uparrow)$, respectively. Making use of Eq. (18), the multi-channel self-energy is equal to

$$\Sigma_3 = \begin{pmatrix} 0 & 0 & 0 & 0 & 0 & 0 & 0 \\ 0 & 0 & 0 & 0 & \frac{U}{2} & 0 & 0 \\ 0 & 0 & 0 & 0 & 0 & 0 & -\frac{U}{2} \\ 0 & 0 & 0 & 0 & 0 & 0 & 0 \\ 0 & \frac{U}{2} & 0 & 0 & 0 & 0 & 0 \\ 0 & 0 & 0 & 0 & 0 & -U & 0 \\ 0 & 0 & -\frac{U}{2} & 0 & 0 & 0 & 0 \end{pmatrix}. \tag{20}$$

The matrix representation of the effective Hamiltonian is

$$H^{\text{eff}} = \begin{pmatrix} \epsilon_0-t & 0 & 0 & 0 & 0 & 0 & 0 \\ 0 & \epsilon_0-t+\frac{U}{2} & 0 & 0 & \frac{U}{2} & 0 & 0 \\ 0 & 0 & \epsilon_0+t+\frac{U}{2} & 0 & 0 & 0 & -\frac{U}{2} \\ 0 & 0 & 0 & \epsilon_0+t & 0 & 0 & 0 \\ 0 & \frac{U}{2} & 0 & 0 & \epsilon_0+3t+\frac{U}{2} & 0 & 0 \\ 0 & 0 & 0 & 0 & 0 & \epsilon_0+t & 0 \\ 0 & 0 & -\frac{U}{2} & 0 & 0 & 0 & \epsilon_0+t+\frac{U}{2} \end{pmatrix}. \tag{21}$$

Solving $[H^{\text{eff}}-\omega]^{-1}$ and calculating the spectral function of the head (a $3\times 3$ block), which corresponds to the 1-GF, we obtain the exact result. The figure in the paper is obtained with $\epsilon_0 = 1$, $t = 1$ and $U = 4$.

### 1/2 filling

The non-interacting (HF) 3-GF in the bonding anti-bonding basis is

$$\begin{aligned} G_{03}(\omega) = \text{Diag}\Big[&\frac{1}{\omega-(\epsilon_0+t+\frac{U}{2})+i\eta}, \frac{1}{\omega-(\epsilon_0+t+\frac{U}{2})+i\eta}, \frac{1}{\omega-(\epsilon_0-t+\frac{U}{2})-i\eta}, \frac{1}{\omega-(\epsilon_0-t+\frac{U}{2})-i\eta}, \\ &\frac{1}{\omega-(\epsilon_0+3t+\frac{U}{2})+i\eta}, \frac{1}{\omega-(\epsilon_0+3t+\frac{U}{2})+i\eta}, \frac{1}{\omega-(\epsilon_0-3t+\frac{U}{2})-i\eta}, \frac{1}{\omega-(\epsilon_0-3t+\frac{U}{2})-i\eta}\Big], \end{aligned} \tag{22}$$

where the first four elements are from the 1-GF with $i = a\downarrow; a\uparrow; b\downarrow; b\uparrow$, respectively, and the last four terms are from $G^{\rm 3p}_{03}$ with $ijl = (a\downarrow a\uparrow b\uparrow); (a\downarrow a\uparrow b\downarrow); (b\downarrow b\uparrow a\uparrow); (b\downarrow b\uparrow a\downarrow)$, respectively. The multi-channel self-energy is equal to

$$\Sigma_3 = \begin{pmatrix} 0 & 0 & 0 & 0 & 0 & 0 & \frac{U}{2} & 0 \\ 0 & 0 & 0 & 0 & 0 & 0 & 0 & -\frac{U}{2} \\ 0 & 0 & 0 & 0 & \frac{U}{2} & 0 & 0 & 0 \\ 0 & 0 & 0 & 0 & 0 & -\frac{U}{2} & 0 & 0 \\ 0 & 0 & \frac{U}{2} & 0 & 0 & 0 & 0 & 0 \\ 0 & 0 & 0 & -\frac{U}{2} & 0 & 0 & 0 & 0 \\ \frac{U}{2} & 0 & 0 & 0 & 0 & 0 & 0 & 0 \\ 0 & -\frac{U}{2} & 0 & 0 & 0 & 0 & 0 & 0 \end{pmatrix}. \tag{23}$$

The effective Hamiltonian is equal to

$$H^{\rm eff} = \begin{pmatrix} \epsilon_0 + t + \frac{U}{2} & 0 & 0 & 0 & 0 & 0 & \frac{U}{2} & 0 \\ 0 & \epsilon_0 + t + \frac{U}{2} & 0 & 0 & 0 & 0 & 0 & -\frac{U}{2} \\ 0 & 0 & \epsilon_0 - t + \frac{U}{2} & 0 & \frac{U}{2} & 0 & 0 & 0 \\ 0 & 0 & 0 & \epsilon_0 - t + \frac{U}{2} & 0 & -\frac{U}{2} & 0 & 0 \\ 0 & 0 & \frac{U}{2} & 0 & \epsilon_0 + 3t + \frac{U}{2} & 0 & 0 & 0 \\ 0 & 0 & 0 & -\frac{U}{2} & 0 & \epsilon_0 + 3t + \frac{U}{2} & 0 & 0 \\ \frac{U}{2} & 0 & 0 & 0 & 0 & 0 & \epsilon_0 - 3t + \frac{U}{2} & 0 \\ 0 & -\frac{U}{2} & 0 & 0 & 0 & 0 & 0 & \epsilon_0 - 3t + \frac{U}{2} \end{pmatrix}. \tag{24}$$

Solving $[H^{\rm eff} - \omega]^{-1}$ and calculating the spectral function of the head (a $4 \times 4$ block), which corresponds to the 1-GF, we obtain the exact result. The figure in the paper is obtained with $\epsilon_0 = -\frac{U}{2}$, $t = 1$ and $U = 4$.


[1] P. Romaniello, S. Guyot, and L. Reining, "The self-energy beyond $GW$: Local and nonlocal vertex corrections," The Journal of Chemical Physics **131** (2009), 10.1063/1.3249965, 154111.

[2] Gabriele Riva, Timothée Audinet, Matthieu Vladaj, Pina Romaniello, and J. Arjan Berger, "Photoemission spectral functions from the three-body Green's function," SciPost Phys. **12**, 093 (2022).
